# Supplementary material for: Learning in a Small/Big World
Source: arXiv:2009.11917 source file (2026-10-21)
Supplement: Supplementary file 1 [file webappendix.tex]

\documentclass[a4paper,12pt]{article}
\usepackage[a4paper, left=2cm, right=2cm, top=3.81cm, bottom=3.81cm]{geometry}
\usepackage{amsmath,xfrac}
\usepackage{xr}
\usepackage{bm}
\usepackage{bbm}
\usepackage{amsthm}
\usepackage{dsfont}
\usepackage[utf8]{inputenc} % added package for displaying German special characters (umlauts)
\usepackage[english]{babel} % added package to display German caption (some issues implementing it)
\usepackage{xcolor} % declare xcolor before tikz
\usepackage{tikz}
\usepackage{adjustbox} %to adjust pictures to framesecon
\usepackage[onehalfspacing]{setspace}
\usepackage{graphicx}
\usepackage{pgfplots}
\usepackage{xcolor, lipsum} % colored boxes
\usepackage{caption}
\usepackage{mathcomp}
\usepackage{verbatim} % comments
\usepackage{enumitem}
\usepackage{listings}
\usepackage[overload]{abraces}
\usepackage{array}
\usepackage{pict2e} 
\usepackage{amssymb}
\usepackage{epstopdf}
\usepackage{pbox}
\usepackage{mathrsfs}
\usepackage{graphicx,wrapfig,lipsum}
\usepackage{multirow}
\usepackage{subcaption}
\usepackage{colortbl}
\usepackage{mathtools}
\usepackage{multicol}
\usepackage{wasysym}
\usepackage{makecell}
\usepackage{eurosym}
\usepackage{booktabs}

\usepackage{pdflscape}
\usepackage{afterpage}
\usepackage{booktabs,arydshln}
\usepackage{capt-of}
\usepackage{rotating}
\usepackage{longtable}
\usepackage{pdfpages}
\usepackage[hidelinks,
colorlinks=true,
urlcolor=blue,
linkcolor=blue,
citecolor=blue,
hyperfootnotes=true]{hyperref}
\usepackage{natbib}
\usepackage{mathtools}

\usetikzlibrary{decorations.pathreplacing}
\usetikzlibrary{positioning, shapes,arrows.meta}
\allowdisplaybreaks[1]

\makeatletter
\newcommand*{\addFileDependency}[1]{% argument=file name and extension
	\typeout{(#1)}
	\@addtofilelist{#1}
	\IfFileExists{#1}{}{\typeout{No file #1.}}
}
\makeatother

\newcommand*{\myexternaldocument}[1]{%
	\externaldocument{#1}%
	\addFileDependency{#1.tex}%
	\addFileDependency{#1.aux}%
}

\myexternaldocument{learning_small_big_world_ver8}

\renewcommand{\ref}[1]{\hyperref[#1]{\ref{#1}}}

\newtheorem{proposition}{Proposition}
\newtheorem{lemma}{Lemma}
\newtheorem{corollary}{Corollary}

\DeclareMathOperator*{\argmax}{arg\,max}

\renewcommand{\thefootnote}{\fnsymbol{footnote}}
\begin{document}
	\onehalfspacing
	\begin{center}
		{\LARGE \textbf{{\LARGE \textbf{Online Appendix of ``Learning in a Small/Big World"}}}}\\
		\vspace{5mm}
		\textit{Benson Tsz Kin Leung\footnote{Hong Kong Baptist University. Email: \href{mailto:btkleung@hkbu.edu.hk}{\texttt{btkleung@hkbu.edu.hk}}, \href{mailto:ltkbenson@gmail.com}{\texttt{ltkbenson@gmail.com}}. }}\\
		\textit{\today}\\
	\end{center}

\onehalfspacing

\renewcommand{\thefootnote}{\arabic{footnote}}
\setcounter{footnote}{0}

\renewcommand\thesection{\Alph{section}}
\setcounter{section}{2}

\renewcommand\theequation{\thesection.\arabic{equation}}
\numberwithin{equation}{section}
\setcounter{equation}{0}
\renewcommand\theproposition{\thesection.\arabic{proposition}}
\numberwithin{proposition}{section}
\setcounter{equation}{0}
\renewcommand\thelemma{\thesection.\arabic{lemma}}
\numberwithin{lemma}{section}
\renewcommand\thecorollary{\thesection.\arabic{corollary}}
\numberwithin{corollary}{section}

\renewcommand\thefigure{\thesection.\arabic{figure}}
\setcounter{section}{0}

	\newtheorem{innercustomgeneric}{\customgenericname}
\providecommand{\customgenericname}{}
\newcommand{\newcustomtheorem}[2]{%
	\newenvironment{#1}[1]
	{%
		\renewcommand\customgenericname{#2}%
		\renewcommand\theinnercustomgeneric{##1}%
		\innercustomgeneric
	}
	{\endinnercustomgeneric}
}
\newcustomtheorem{assumption}{Assumption}

\begin{center}
	\Large \textbf{For online publication only}
\end{center}

\section{Switching between different automatons}\label{section:switch}
This section illustrates how the setup in this paper encompasses learning mechanisms that involve switching between automatons with size smaller than $M$. 

I first argue that assuming that the DM could switch between multiple learning mechanisms with $M$ memory states implicitly implies that he has a larger memory capacity than $M$. Suppose that a DM starts with $(\mathscr{T},d)$ at memory state $m_{1}$ and switches to $(\mathscr{T}',d')$ and $(\mathscr{T}'',d'')$ once he transit to memory state $m_{1}$ and $m_{2}$ respectively. As $(\mathscr{T},d)\neq(\mathscr{T}',d')\neq(\mathscr{T}'',d'')$, when the DM receives a signal $s$ at memory state $m$ and decides to which memory state he transit to, or when he decides which action he takes at memory state $m$, he has to remember whether he has once transited to memory state $m_{1}$ and $m_{2}$. In other words, the DM has to track not only his current memory states, but also has to memorize the (incomplete) history of his previous memory states. Switching between multiple automatons thus implicitly implies a larger memory capacity.

Now, I illustrate through an example that a $M$ memory states automaton could be designed to involve switching between automatons with smaller sizes. The example is illustrated in Figure~\ref{fig:switch}. In this example, the DM starts at memory state $3$ with a learning mechanism $(\mathscr{T},d)$ that involves 5 memory states $1$ to $5$. Once he transits to memory state $1$, he switches to another learning mechanism $(\mathscr{T}',d')$ that involves 5 memory states $1$, $10, 11, 12, 13$. On the other hand, once he transits to memory state $5$, he switches to the learning mechanism $(\mathscr{T}',d')$ that involves 5 memory states $5, 6, 7, 8, 9$. Thus, the proposed 13 memory states automaton can be interpreted as a mechanism that involves switching between three 5 memory states automatons.

\tikzstyle{cloud} = [draw, align=left, circle,fill=cyan!20, node distance=3cm,
minimum height=1em]
\tikzstyle{cloud1} = [draw, align=left, circle,fill=black, node distance=1cm,
minimum height=0.01cm]
\tikzstyle{cloud2} = [draw, align=left, circle,fill=red, node distance=1cm,
minimum height=0.01cm]
\tikzset{
	dot/.style = {circle, fill, minimum size=#1,
		inner sep=0pt, outer sep=0pt},
	dot/.default = 3pt % size of the circle diameter 
}

\begin{figure}
	\centering
	\begin{tikzpicture}[every text node part/.style={align=center}]
		\node[cloud] (m1) {\footnotesize 1};
		\node[cloud, right = 3em of m1] (m2) {\footnotesize 2};
		\node[cloud, right = 3em of m2] (m3) {\footnotesize 3};
		\node[above = 3em of m3, align=center] (m0) {Initial \\memory state};
		\node[cloud, right = 3em of m3] (m4) {\footnotesize 4};
		\node[cloud, right = 3em of m4] (m5) {\footnotesize 5};
		\node[cloud, fill=red!60, above right= 2em and 2em of m5] (m6) {\footnotesize 6};
		\node[cloud, fill=red!60, above right= 2em and 2em of m6] (m7) {\footnotesize 7};
		\node[cloud, fill=red!60, below right= 2em and 2em of m5] (m8) {\footnotesize 8};
		\node[cloud, fill=red!60, below right= 2em and 2em of m8] (m9) {\footnotesize 9};
		\node[cloud, fill=green!40, above left= 2em and 2em of m1] (m10) {\footnotesize 10};
		\node[cloud, fill=green!40, above left= 2em and 2em of m10] (m11) {\footnotesize 11};
		\node[cloud, fill=green!40, below left= 2em and 2em of m1] (m12) {\footnotesize 12};
		\node[cloud, fill=green!40, below left= 2em and 2em of m12] (m13) {\footnotesize 13};
		\node[below left = 2em and 0.05em of m1] (1below) {};
		\node[below right = 2em and 0.05em of m5] (5below) {};
		\draw [decorate,decoration={brace,mirror,amplitude=5pt},xshift=0pt,yshift=0pt]
		(1below) -- (5below) node [black,midway,yshift=-0.6cm]
		{\footnotesize $(\mathscr{T},d)$};
		\node[below right = 1em and 0.05em of m9] (9below) {};
		\node[below left = 7.5em and 0.05em of m5] (5below') {};
		\draw [decorate,decoration={brace,mirror,amplitude=5pt},xshift=0pt,yshift=0pt]
		(5below') -- (9below) node [black,midway,yshift=-0.6cm]
		{\footnotesize $(\mathscr{T}'',d'')$};
		\node[below right = 8em and 0.05em of m1] (1below') {};
		\node[below left = 1em and 0.05em of m13] (13below) {};
		\draw [decorate,decoration={brace,mirror,amplitude=5pt},xshift=0pt,yshift=0pt]
		(13below) -- (1below') node [black,midway,yshift=-0.6cm]
		{\footnotesize $(\mathscr{T}',d')$};
		\draw[-Latex]
		(m0) edge (m3)
		(m2) edge[bend right] node [below, midway] {} (m3)
		(m3) edge[bend right] node [below, midway] {} (m4)
		(m4) edge[bend right] node [above, midway] {} (m3)
		(m3) edge[bend right] node [above, midway] {} (m2)
		(m2) edge[bend right] node [above, midway] {} (m1)
		(m4) edge[bend left] node [above, midway] {} (m5)
		(m1) edge[bend left] node [above, midway] {} (m10)
		(m10) edge[bend left] node [above, midway] {} (m11)
		(m10) edge[bend left] node [above, midway] {} (m1)
		(m11) edge[bend left] node [above, midway] {} (m10)
		(m1) edge[bend left] node [above, midway] {} (m12)
		(m12) edge[bend left] node [above, midway] {} (m13)
		(m12) edge[bend left] node [above, midway] {} (m1)
		(m13) edge[bend left] node [above, midway] {} (m12)
		(m5) edge[bend left] node [above, midway] {} (m6)
		(m6) edge[bend left] node [above, midway] {} (m7)
		(m5) edge[bend left] node [above, midway] {} (m8)
		(m8) edge[bend left] node [above, midway] {} (m9)
		(m6) edge[bend left] node [above, midway] {} (m5)
		(m7) edge[bend left] node [above, midway] {} (m6)
		(m8) edge[bend left] node [above, midway] {} (m5)
		(m9) edge[bend left] node [above, midway] {} (m8);
		%(m1) edge[loop above,looseness=10] node [left] {} (m1)
		%(m4) edge[loop above,looseness=10] node [right] {} (m4);
	\end{tikzpicture}
	\caption{An example of a 13 memory states automaton that involves switching between three 5 memory states automatons. The DM starts at memory state $3$ with $(\mathscr{T},d)$, and switches to $(\mathscr{T}',d')$ and $(\mathscr{T}'',d'')$ once he transits to memory state $1$ and $5$, respectively.}
	\label{fig:switch}
\end{figure}

\section{Discounted future utility}\label{section:wilson}
In this section, I looked into the alternative formulation where future utility are discounted. More specifically, we look into the following updating mechanism
\begin{equation*}
	(m^{*D}_1(\rho),\mathscr{T}^{*D}(\rho),d^{*D}(\rho))=\argmax_{m_1,\mathscr{T},d} E\left[(1-\rho)\sum_{t=1}^{\infty}\rho^t u(a_t,\omega)\right],
\end{equation*}
for some discount factor $\rho<1$. We have the following result.
\begin{proposition}\label{prop_discountfactor}
	For all $\epsilon>0$, there exists some $\bar{\rho}<1$ such that $L(m^{*D}_1(\rho),\mathscr{T}^{*D}(\rho),d^{*D}(\rho))<L^*_M+\epsilon$ for all $\rho>\bar{\rho}$.
\end{proposition}
In other words, for $\rho$ close to $1$, the updating mechanism that maximizes discounted sum of utility, $(m^{*D}_1(\rho),\mathscr{T}^{*D}(\rho),d^{*D}(\rho))$, is also $\epsilon$-optimal for very small $\epsilon$. Thus, the results in the main text continues to hold.

	\section{An example of ignorance with uniform prior belief and symmetric signal structures}\label{sec:symmetric}
In this section,% I present an example that shows that not only the prior belief and signal distributions, but also the complexity of the world plays a role in the optimality of ignorant learning behaviors. In particular, ignorance could be optimal in a setting with symmetric prior belief and signal distributions when $N$ is big enough or when the signal distributions are uninformative enough.
I consider a case where $N=M\geq 4$ and states of the world are a priori uniformly distributed, i.e., $p^{\omega}=\frac{1}{N}$ for all $\omega=\lbrace 1,\cdots, N\rbrace$. Moreover, $u(\omega,\omega)=1>u(\omega',\omega)=0$ for all $\omega$ and $\omega'\neq\omega$. For  simplicity, consider a class of ``symmetric" discrete signal structures where $S=\lbrace s^{1},\cdots.s^{N}\rbrace$ and $s^{\omega}$ is a signal that supports state $\omega$. More specifically,
\begin{equation*}
	F^{\omega}(s^{\omega})=\mathscr{I}F^{\omega}(s^{\omega'}) \text{ for all $\omega$ and $\omega'\neq\omega$ where $\mathscr{I}>1$.}
\end{equation*} 
Thus, under all states of the world, it is $\mathscr{I}$ times more likely to receive a signal that supports the true state than a signal that supports one of the other states.

In such a symmetric environment, there seems to be no reason to ignore any of the states. However, I will present an example that shows that it is beneficial to ignores some states when $N$ is large or $\mathscr{I}$ is small. First, consider a simple ``symmetric" updating mechanism that ignores no states, illustrated in Figure~\ref{fig:symmetricallstates1appendix} with an example of $N=4$. As the DM ignores no state, he allocates one memory state to each action. Without loss of generality, assume he takes action~$\omega$ in memory state $\omega$. When the DM is in memory state $m=\omega$, upon receiving a signal $s^{\omega'}$, i.e., a signal that supports state $\omega'$, he transits to memory state $\omega'$ with some probability $\delta_{m\omega}\leq1$, and stays in his current memory state otherwise. Formally, the transition function is as follows:
\begin{equation*}
	\mathscr{T}(m,s^{\omega})=\delta_{m\omega}\times \lbrace\omega\rbrace+(1-\delta_{m\omega})\times \lbrace m\rbrace \text{ for all $m$ and $\omega$.}
\end{equation*}
In the following I show that such updating mechanism is optimal among the class of all non-ignorant mechanism.

Suppose for some non-ignorant mechanism that the DM chooses action~$\omega$ in memory state $m=\omega$, and the DM transits from memory state $m$ to memory state $\omega$ upon receiving signal $s^{\omega'}$ with strictly positive probability where $\omega'\neq\omega'$. Similar to the proof of Proposition~\ref{prop_smallworld} (i), I construct an updating mechanism that strictly improves asymptotic utility. First, decrease the probability of transiting from memory state $m$ to $\omega$ upon receiving signal $s^{\omega'}$ by $p$. Second, increase the probability of transiting from memory state $m$ to $\omega$ upon receiving signal $s^{\omega}$ by $p$ (re-normalize if necessary). These two steps do not change the utility in all state $\omega''\neq \omega,\omega'$, increase the utility in state $\omega$ but decrease the utility in state $\omega'$. Last, scale up all the transitions out of memory state $\omega$ (re-normalize if necessary) such that the utility in state $\omega$ is the same before the first step of construction. As it is less likely to receive $s^{\omega}$ in state $\omega'$ than in state $\omega$, the last step ``over-scale-up"  the transition out of memory state $\omega$, and thus increases the utility in state $\omega'$ such that it is higher before the construction.

\begin{comment}
Suppose state $1$ is true, in the stationary distribution, we have
\begin{equation*}
	\begin{split}
		\delta\mu^{1}_{\omega}\sum_{\omega'\neq\omega}F^{1}(s^{\omega'})&=\delta F^{1}(s^{\omega})\sum_{\omega'\neq\omega}\mu^{1}_{\omega'}\text{ for all $\omega$.}
	\end{split}
\end{equation*}
It is easy to see that the solution of the system of equations satisfy:
\begin{equation*}
	\begin{split}
		\mu^{1}_{1}F^{1}(s^{\omega})=\mu^{1}_{\omega}F^{1}(s^{1}) \text{ for all $\omega\neq 1$,}
	\end{split}
\end{equation*}
which says that all probability mass going out from memory state $1$ to memory state~$\omega$ must be equal to that going from memory state $\omega$ to memory state $1$. Thus $\mu^{1}_{1}=\mathscr{I}\mu^{1}_{\omega}$ for all $\omega\neq 1$, and $\mu^{1}_{1}=\frac{\mathscr{I}}{N+\mathscr{I}-1}$. By repeating the same procedure for other states of the world, the asymptotic utility of this symmetric non-ignorant updating mechanism equals:
\begin{equation}
	\sum_{\omega=1}^{N}\frac{\mathscr{I}}{N+\mathscr{I}-1}\frac{1}{N}=\frac{\mathscr{I}}{N+\mathscr{I}-1}
	\label{eq:losssymmetric}
\end{equation}
which decreases in $N$. When $N$ is large, it is very easy for the DM to receive one signal that supports the wrong state and makes a mistake, i.e., the updating mechanism is ``noisier".
\end{comment}

	\begin{figure}
	\centering
	\begin{tikzpicture}[every text node part/.style={align=center}]
		\node[cloud] (m1) {\footnotesize 1};
		\node[cloud, right = 10em of m1] (m2) {\footnotesize 2};
		\node[cloud, below = 10em of m1] (m3) {\footnotesize 3};
		\node[cloud, below = 10em of m2] (m4) {\footnotesize 4};
		\draw[-Latex]
		(m1) edge[bend right=10] node [left, midway] {\footnotesize$\delta_{13}\times S_{3}$} (m3)
		(m3) edge[bend right=10] node [right, midway] {\footnotesize$\delta_{31}\times  S_{1}$} (m1)
		(m1) edge[bend right=10] node [below, midway] {\footnotesize$\delta_{12}\times S_{2}$} (m2)
		(m2) edge[bend right=10] node [above, midway] {\footnotesize$\delta_{21}\times S_{1}$} (m1)
		(m2) edge[bend right=10] node [left, midway] {\footnotesize$\delta_{24}\times S_{4}$} (m4)
		(m4) edge[bend right=10] node [right, midway] {\footnotesize$\delta_{42}\times S_{2}$} (m2)
		(m3) edge[bend right=10] node [below, midway] {\footnotesize$\delta_{34}\times S_{4}$} (m4)
		(m4) edge[bend right=10] node [above, midway] {\footnotesize$\delta_{43}\times S_{3}$} (m3)
		(m2) edge[bend right=90, looseness=2] node [above left, midway] {\footnotesize$\delta_{23}\times S_{3}$} (m3)
		(m3) edge[bend right=90, looseness=2] node [below right, midway] {\footnotesize$\delta_{32}\times S_{2}$} (m2)
		(m1) edge[bend right=90, looseness=2] node [below left, midway] {\footnotesize$\delta_{14}\times S_{4}$} (m4)
		(m4) edge[bend right=90, looseness=2] node [above right, midway] {\footnotesize $\delta_{41}\times S_{1}$} (m1);
	\end{tikzpicture}
	\caption{The optimal non-ignorant updating mechanism that considers all states, with $N=M=4$. The number in the node denotes the action that the DM takes when he is this memory state. Moreover, in memory state $\omega$, and upon receiving a signal that supports state~$\omega'\neq\omega$, the DM transits to memory state~$\omega'$ with probability $\delta_{\omega\omega'}<1$ and stays in his current memory state otherwise.}
	\label{fig:symmetricallstates1appendix}
\end{figure}

\begin{figure}
	\centering
	\begin{tikzpicture}[every text node part/.style={align=center}]
		\node[cloud] (m1) {\footnotesize 1};
		\node[cloud, right = 5em of m1] (m2) {\footnotesize 2};
		\node[cloud, right = 5em of m2] (m3) {\footnotesize 3};
		\node[cloud, right = 5em of m3] (m4) {\footnotesize 4};
		\draw[-Latex]
		(m1) edge[bend right=10] node [below, midway] {\footnotesize$\delta\times S_{2}$} (m2)
		(m2) edge[bend right=10] node [above, midway] {\footnotesize$ S_{1}$} (m1)
		(m2) edge[bend right=10] node [below, midway] {\footnotesize$\delta\times S_{2}$} (m3)
		(m3) edge[bend right=10] node [above, midway] {\footnotesize$\delta\times S_{1}$} (m2)
		(m3) edge[bend right=10] node [below, midway] {\footnotesize$S_{2}$} (m4)
		(m4) edge[bend right=10] node [above, midway] {\footnotesize$\delta\times S_{1}$} (m3);
	\end{tikzpicture}
	\caption{An example of an updating mechanism that ignore two states, with $N=M=4$. The DM takes action $1$ in memory states $1$ and $2$, and takes action~$2$ in memory states $3$ and $4$. In memory state~$3$, if the DM receives a signal supporting state~$2$, he transits to memory state~$4$; if the DM receives a signal supporting state~$1$, he transits to memory state~$2$ with probability $\delta$ and stays in his current memory state otherwise. In memory state~$4$, if the DM receives a signal state~$1$, he transits to memory state~$3$ with probability $\delta$  and stays in his current memory state otherwise. The transition function in memory state~$1$ and $2$ are defined accordingly. $\delta$ is chosen to be close to $0$ to maximize the asymptotic utility.}
	\label{fig:symmetricignorestates1appendix}
\end{figure}

Now consider an ignorant mechanism that follows the similar idea of the non-ignorant updating mechanism illustrated in Figure~\ref{fig:symmetricallstates1appendix}, but ignores half of the states of the worlds. For simplicity, assume that $N$ is plural. The ignorant mechanism is illustrated in Figure~\ref{fig:symmetricignorestates1appendix}, with an example of $N=4$. By ignoring half of the states, the DM allocates two memory states to each action that he does not  ignore. Without loss of generality, assume that the DM takes action~$\omega$ in memory states $2\omega-1$ and $2\omega$ for $\omega\leq\frac{N}{2}$, and ignores all actions $\omega'>\frac{N}{2}$. In the ``more confident" memory state $2\omega$, upon receiving a signal supporting state $\omega'\neq\omega$ where $\omega'\leq \frac{N}{2}$, the DM transits to state $2\omega-1$ with probability $\delta<1$ and stays in his current memory state otherwise. In the ``less confident" memory state $2\omega-1$, upon receiving a signal that supports state $\omega$, he transits to the ``more confident" memory state $2\omega$; upon receiving a signal that supports state $\omega'\neq\omega$ where $\omega'\leq \frac{N}{2}$, the DM transits to state $2\omega'-1$ with probability $\delta<1$ and stays in his current memory state otherwise.

Formally, the transition function is as follows:
\begin{small}
	\begin{alignat*}{2}
		\mathscr{T}(2\omega,s^{\omega})&= 2\omega  &&\text{ for all $\omega\leq\frac{N}{2}$,}\\
		\mathscr{T}(2\omega,s^{\omega'})&=\begin{cases}
			2\omega-1 \text{ with probability $\delta$}\\
			2\omega  \text{ with probability $1-\delta$}
		\end{cases}
		&&\text{ for all $\omega\leq\frac{N}{2}$, $\omega'\neq\omega$ and $\omega'\leq\frac{N}{2}$,}\\
		\mathscr{T}(2\omega-1,s^{\omega})&= 2\omega  &&\text{ for all $\omega\leq\frac{N}{2}$,}\\
		\mathscr{T}(2\omega-1,s^{\omega'})&=\begin{cases}
			2\omega'-1 \text{ with probability $\delta$}\\
			2\omega  \text{ with probability $1-\delta$}
		\end{cases} &&\text{ for all $\omega\leq\frac{N}{2}$, $\omega'\neq\omega$ and $\omega'\leq\frac{N}{2}$,}\\
		\mathscr{T}(m,s^{\omega'})&= m &&\text{ for all $\omega>\frac{N}{2}$.}
	\end{alignat*}
\end{small}
Suppose the true state is $1$, In the stationary distribution, we must have
\begin{equation}
	\begin{split}
		\delta\mu^{1}_{2\omega}\sum_{\omega'\neq\omega,\omega'\leq\frac{N}{2}}F^{1}(s^{\omega'})&=\mu^{1}_{2\omega-1}F^{1}(s^{\omega})\text{ for all $\omega\leq\frac{N}{2}$,}\\
		\delta\mu^{1}_{2\omega-1}F^{1}(s^{\omega'})&=\delta\mu^{1}_{2\omega'-1}F^{1}(s^{\omega})\text{ for all $\omega,\omega'\leq\frac{N}{2}$ and $\omega\neq\omega'$.}
	\end{split}
	\label{eq:ignorehalfstate}
\end{equation}
From the first Equation of Equation~\ref{eq:ignorehalfstate}, we know that when $\delta$ is close to $0$, $\mu^{1}_{2\omega-1}$ is close to $0$ for all $\omega\leq\frac{N}{2}$. Moreover, we have
\begin{equation*}
	\begin{split}
		\mu^{1}_{2}&=\frac{F^{1}(s^{1})}{\delta\sum_{\omega'\neq1,\omega'\leq\frac{N}{2}}F^{1}(s^{\omega'})}\times\frac{\delta F^{1}(s^{1})}{\delta F^{1}(s^{\omega})}\times \frac{\delta\sum_{\omega'\neq\omega,\omega'\leq\frac{N}{2}}F^{1}(s^{\omega'})}{F^{1}(s^{\omega})}\times\mu^{1}_{2\omega}\\
		&=\frac{\mathscr{I}}{\frac{N}{2}-1}\times\mathscr{I}\times\left(\frac{N}{2}-2+\mathscr{I}\right)\times\mu^{1}_{2\omega}\\
		&=\frac{\mathscr{I}^{2}(N+2\mathscr{I}-4)}{N-2}\mu^{1}_{2\omega}
	\end{split}
\end{equation*} 
for all $\omega\neq1$ and $\omega\leq\frac{N}{2}$. We have
\begin{equation*}
	\begin{split}
		\mu^{1}_{2}+\sum_{\omega\neq 1,\omega\leq\frac{N}{2}}\mu^{1}_{2\omega}&=1\\
		\mu^{1}_{2}+\frac{N-2}{\mathscr{I}^{2}(N+2\mathscr{I}-4)}\left(\frac{N}{2}-1\right)\mu^{1}_{2}&=1\\
		\mu^{1}_{2}&=\frac{2\mathscr{I}^{2}(N+2\mathscr{I}-4)}{2\mathscr{I}^{2}(N+2\mathscr{I}-4)+(N-2)^{2}}.
	\end{split}
\end{equation*}
By repeating the same computation for all $\omega\leq\frac{N}{2}$, the asymptotic utility equals:
\begin{equation}
	\sum_{\omega=1}^{\frac{N}{2}}\frac{2\mathscr{I}^{2}(N+2\mathscr{I}-4)}{2\mathscr{I}^{2}(N+2\mathscr{I}-4)+(N-2)^{2}}\times\frac{1}{N}=\frac{\mathscr{I}^{2}(N+2\mathscr{I}-4)}{2\mathscr{I}^{2}(N+2\mathscr{I}-4)+(N-2)^{2}}.
\end{equation}
Then the R code on \url{https://sites.google.com/site/ltkbenson/research} produces Figure~\ref{fig:compareignoreornonignorant} in the main text.

\section{Infinite $N$}\label{section:infinite}
In this section, I analyze an extension where $N,M\rightarrow\infty$ and characterize a sequence of updating mechanism $\mathscr{T}_{N,M}$ that is $\epsilon$-optimal at the limit where $N,M\rightarrow\infty$. Moreover, I focus on cases where $N=\Theta(M^{h})$, i.e., $N$ goes to infinite as fast as $M^{h}$. In this setting, small worlds refer to the case where $h<1$ and big worlds refer to the case where $h\geq 1$. Note that when $h<1$, as $N,M\rightarrow\infty$, $\frac{N}{M}\rightarrow 0$; when $h\geq 1$, $\lim_{N,M\rightarrow\infty}\frac{N}{M}> 0$. In the following, I show that the results in the baseline model hold qualitatively in this extension. %In the baseline model where $N$ is fixed and finite, it is difficult to analyze the effects of a change in complexity $N$, as the prior beliefs and thus the importance of identifying different states also changes with $N$. Consequently, to 
It thus shows that the behavioral implications depend on both $N$ and $M$, and more specifically the ratio $\frac{N}{M}$, instead of just the absolute value of $M$. %It thus shows that the characteristics of learning behaviors depend on whether the ratio $\frac{N}{M}$ is close to or bounded away from $0$ but not on whether $M$ goes to infinite or not.

Formally, I consider a sequence of inference problems, which are characterized by the utilities, prior beliefs and information structures, i.e., $ \lbrace (\bm{u}^{\omega}_{N},p^{\omega}_{N},f^{\omega}_{N})_{\omega=1}^{N}\rbrace_{N=1}^{\infty}$. The subscript $N$ emphasizes the fact that the utilities, prior beliefs, and information structures could change along the sequence. A small world is a sub-sequence of inference problems with a sequence of  memory size $M$, and is denoted by $\left\lbrace (\bm{u}^{\omega}_{N(k)},p^{\omega}_{N(k)},f^{\omega}_{N(k)})_{\omega=1}^{N(k)},M(k)\right\rbrace_{k=1}^{\infty}$ where $\lim_{k\rightarrow\infty}N(k),M(k)\rightarrow\infty$ and $N(k)=\Theta(M(k)^{h})$ with $h<1$. For example, $N(k)=k$ and $M(k)=k^2$, such that the sequence $M(k)$ dominates the sequence $N(k)$ at the limit. A big world is defined analogously with $h\geq 1$. For ease of exposition, I sometimes omit the argument $k$ in the sequences $N(k)$ and $M(k)$.
%I first examine whether learning is close to Bayesian at the limit, i.e., whether $\lim_{N,M\rightarrow \infty}L^{*}_{NM}=0$ given the sequence $\left\lbrace (\bm{u}^{\omega}_{N},p^{\omega}_{N},f^{\omega}_{N})_{\omega=1}^{N}\right\rbrace_{N=1}^{\infty}$. Second, I evaluate whether a sequence of updating mechanisms $\lbrace\mathscr{T}_{N}\rbrace_{N=1}^{\infty}$ that ignores some states at the limit could be optimal when $N,M\rightarrow\infty$. Third, I investigate whether two individuals who adopt a sequence of $\epsilon$-optimal mechanisms with small $\epsilon$ could disagree with each other asymptomatically as $N,M\rightarrow\infty$.

Before I present the result, it is necessary to present some additional assumptions about the nature of the sequence of inference problems. First, I assume that $u_{N}(\omega,\omega)-\max_{\omega'\neq\omega}u_{N}(\omega',\omega)\in[\underline{u},\overline{u}]$ for some $\underline{u}>0$ for all $\omega$ and all $N$. Thus along the sequence of inference problems, no states are infinitely more important than another state. The prior belief of the DM satisfies the following full support assumption:
\begin{assumption}{D.1}\label{assumption_fullsupportinfinite}
	For any sequence of subset of states $\Omega_{N}\subseteq
	\lbrace 1,\cdots, N\rbrace$ with cardinality $\vert\Omega_{N}\vert$ and a well-defined limit $\lim_{N\rightarrow \infty}\frac{\vert\Omega_{N}\vert}{N}$, 
	\begin{equation}
		\lim_{N\rightarrow \infty}\sum_{\omega\in\Omega_{N}}p_{N}^{\omega}>0\text{ if $\lim_{N\rightarrow \infty}\frac{\vert\Omega_{N}\vert}{N}>0$.}
		\label{eq:fullsupportinfinite}
	\end{equation}
\end{assumption}
That is, Equation~\eqref{eq:fullsupportinfinite} ensures any sequence of subsets of states that has a non-negligible measure in fractions at the limit, i.e., $\lim_{N\rightarrow \infty}\frac{\vert\Omega_{N}\vert}{N}>0$, also has a non-negligible probability mass at the limit, i.e., $\lim_{N\rightarrow \infty}\sum_{\omega\in\Omega_{N}}p_{N}^{\omega}>0$.\footnote{For example, it rules out prior beliefs $(p_N^{\omega})_{\omega=1}^{N}$ where $p^{\omega}=\frac{1}{N^{2}}$ for $\omega\leq \frac{N}{2}$ and  $p^{\omega}=\frac{2N-1}{N^{2}}$ for $\omega>\frac{N}{2}$, i.e., first half of all possible states have negligible probability mass at  the limit.} This is analogue to the full support assumption in the baseline model. A simple example would be $p^{\omega}_{N}=\frac{1}{N}$ for all $\omega$ and $N$.

Similar to the baseline model, I assume that no signals rule out any states of the world: there exists $\varsigma>0$ such that
\begin{equation}\label{assumption_noperfectsignalinfinite}
	\inf_{s\in S}\frac{f_{N}^{\omega}(s)}{f_{N}^{\omega'}(s)}>\varsigma \text{ for all $\omega$, $\omega'\in \Omega$ and for all $N$}.
\end{equation}
Finally, I make the following assumption about identifiability that plays similar role to the assumption that $f^{\omega}\neq f^{\omega'}$ in the baseline model. It ensures that signal structures with negligible Cauchy-Schwarz distances must have negligible probability mass at the limit.

\begin{assumption}{D.2}\label{assumption_identifiableinfinte}
	For all $\varepsilon>0$, there exists some $\xi>0$ and some sequence of subsets of states $N_{\xi}\subseteq	\lbrace 1,\cdots, N\rbrace$ such that $\lim_{N\rightarrow\infty}\left(\sum_{\omega\in N_{\xi}}p_{N}^{\omega}\right)>1-\varepsilon$ and
	\begin{equation*}
		\lim_{N\rightarrow\infty}\inf_{\omega,\omega'\in N_{\xi}; \omega'\neq\omega}\left\lbrace-\log\dfrac{\int f_{N}^{\omega}(s)f_{N}^{\omega'}(s)ds}{\sqrt{\int (f_{N}^{\omega}(s))^{2}ds}\sqrt{\int (f_{N}^{\omega'}(s))^{2}ds}}\right\rbrace>\xi,
	\end{equation*}
\end{assumption}
Appendix~\ref{section:signalstructure} provides an example of the signal structures that satisfy Assumption~\ref{assumption_identifiableinfinte} and Equation~\ref{assumption_noperfectsignalinfinite}. Analogue to the main text, $L^*_k$ denotes the infinmum of the asymptotic utility loss with $N(k)$ and $M(k)$, $\lim_{k\rightarrow\infty}L^*_k$ denotes the infinmum of the asymptotic utility as $k$ goes to infinite, and a sequence of updating mechanism $\lbrace (m_{1k},\mathscr{T}_k,d_{k})\rbrace_{k=1}^{\infty}$ is $\epsilon$-optimal (at the limit) if $\lim_{k\rightarrow\infty}L_k(m_{1k},\mathscr{T}_k,d_{k})\leq \lim_{k\rightarrow\infty}L^*_k+\epsilon$. %Also denote the set of sequence of $\epsilon$-optimal updating mechanism as $\pmb{\mathscr{T}^{\epsilon}_{\infty}}$.%, i.e., the assumption that no signals rule out any states and almost all states are identifiable.

\subsection{Small Worlds}
First, I present the results in small worlds. The following proposition shows that actions taken by the DM is close to the Bayesian benchmark.
\begin{proposition}\label{prop_smallworldinfiniteN}
	Fix $\left\lbrace (\bm{u}^{\omega}_{N(k)},p^{\omega}_{N(k)},f^{\omega}_{N(k)})_{\omega=1}^{N(k)},M(k)\right\rbrace_{k=1}^{\infty}$ where $N(k)=\Theta(M_{i}(k)^{h_{i}})$ with $h<1$. For all $\epsilon>0$, there exists a sequence of updating mechanism $\lbrace m_{1k},\mathscr{T}_{k},d_{k}\rbrace_{k=1}^{\infty}$ such that $\lim_{k\rightarrow\infty}L(m_{1k},\mathscr{T}_{k},d_{k})<\epsilon$. Therefore, $\lim_{k\rightarrow\infty}L^*_k=0$
\end{proposition}
The intuition and the proof of the proposition follow similar arguments in Proposition~\ref{prop_smallworld}. In particular, I show that the simple updating mechanism illustrated in Figure~\ref{fig:simplelearningalgosmallworld} achieves perfect asymptotic learning. Similar to the baseline model, as $\frac{M}{N}\rightarrow\infty$, the DM could allocate infinite memory states to each state, and his confidence level for each action ranges from $1$ to $\infty$. As the DM could be almost sure about taking each action, he makes no mistakes asymptotically and he almost always matches his action with the true state. 

Next, as the DM can learn perfectly under every state of the world, he has no incentive to ignore some states of the world to focus on a strict subset of states, i.e., ignorance in learning is not optimal.
\begin{corollary}\label{coro_ignorancesmallworldinfinteN}
	Fix $\left\lbrace (\bm{u}^{\omega}_{N(k)},p^{\omega}_{N(k)},f^{\omega}_{N(k)})_{\omega=1}^{N(k)},M(k)\right\rbrace_{k=1}^{\infty}$ where $N(k)=\Theta(M(k)^{h})$ with $h<1$. A sequence of updating mechanisms $\lbrace m_{1k},\mathscr{T}_{k},d_{k}\rbrace_{k=1}^{\infty}$ is $\epsilon$-optimal at the limit $k\rightarrow \infty$ only if it ignores at most $\frac{\epsilon}{\underline{u}}$ measures of states at the limit.
\end{corollary}
In particular, when $\epsilon\rightarrow 0$, Corollary~\ref{coro_ignorancesmallworldinfinteN} shows that the optimal updating mechanism must ignore at most a negligible amount of states. To complete the analysis in small worlds, the following corollary shows that different individuals are bound to agree in small worlds if they agree on the probability $0$ events.\footnote{Note that in the baseline model, individuals necessarily agree on the probability $0$ events as $p^{\omega}>0$ for all $\omega$. In contrast, Assumption~\ref{assumption_fullsupportinfinite} does not guarantee an agreement: there may exist some $\omega$ such that $\lim_{N\rightarrow \infty}p^{\omega}_{NA}>0$ but $\lim_{N\rightarrow \infty}p^{\omega}_{NB}=0$.}

\begin{corollary}\label{coro_agreesmallworld1infiniteN}
	Fix $\left\lbrace (\bm{u}^{\omega}_{N(k)i},p^{\omega}_{N(k)i},f^{\omega}_{N(k)i})_{\omega=1}^{N(k)},M_{i}(k)\right\rbrace_{k=1}^{\infty}$ where $N(k)=\Theta(M_{i}(k)^{h_{i}})$ with $h_i<1$ for $i=A,B$. If $\lim_{N\rightarrow\infty}p^{\omega}_{NA}>0$ if and only if $\lim_{N\rightarrow\infty}p^{\omega}_{NB}>0$ for all $\omega\in\lbrace 1,\cdots\infty\rbrace$, individual A and B must almost always agree with each other at the limit if they adopt a sequence of $\epsilon$-optimal updating mechanism with $\epsilon\rightarrow 0$.
	
	%we have
	%\begin{equation*}
		%\lim_{k\rightarrow\infty}\lim_{\epsilon\rightarrow 0}\sum_{\omega}\left[\mathbbm{1}\left\lbrace\lim_{T\rightarrow \infty}E_{\omega,\mathscr{T}_{kA},\mathscr{T}_{kB}}\frac{\sum_{t=1}^{T}\mathbbm{1}_{a^A_t=a^B_t}}{T}=1\right\rbrace p^{\omega}_{Ni}\right]=1 \text{ for all $\lbrace\mathscr{T}_{ki}\rbrace_{k=1}^{\infty}\in\pmb{\mathscr{T}_{\infty i}^{\epsilon}}$ and $i=A,B$}. 
	%\end{equation*}
\end{corollary}

\subsection{Big Worlds}
Now I present the results in big worlds. First, the following Proposition shows that asymptotic learning is different than Bayesian.
\begin{proposition}\label{prop_bayesianlearningbigworldinfiniteN}
	Fix $\left\lbrace (\bm{u}^{\omega}_{N(k)},p^{\omega}_{N(k)},f^{\omega}_{N(k)})_{\omega=1}^{N(k)},M(k)\right\rbrace_{k=1}^{\infty}$ where $N(k)=\Theta(M(k)^{h})$ with $h\geq1$, $\lim_{k\rightarrow\infty}L_{k}^{*}>0$. 
\end{proposition}
The intuition is again similar to Proposition~\ref{prop_smallworld} in the baseline model. In this extension, similar to the baseline model, $\frac{M}{N}<\infty$ implies that the DM can only allocate a finite number of memory states to almost all states of the world. However, to make no mistakes when choosing action~$\omega$, the DM has to record infinite signals supporting state~$\omega$ and be almost sure about state~$\omega$. As $\frac{M}{N}<\infty$ is bounded, the DM cannot be allocate infinite number of memory states to record supporting information for each state of the world. Thus he cannot be almost sure for almost all actions and is bound to make mistakes. Next, I show the analogue of Proposition~\ref{prop_bigworldignorance2} about ignorance in this extension. 

\begin{proposition}\label{prop_bigworldignorance2infiniteN}
	Fix $\left\lbrace (\bm{u}^{\omega}_{N(k)},p^{\omega}_{N(k)},f^{\omega}_{N(k)})_{\omega=1}^{N(k)},M(k)\right\rbrace_{k=1}^{\infty}$ where $N(k)=\Theta(M(k)^{h})$ with $h\geq1$. All updating mechanisms must ignore almost all (measured in fraction) states at the limit.
\end{proposition}

Note that the statements in Proposition~\ref{prop_bigworldignorance2} and~\ref{prop_bigworldignorance2infiniteN} are different. Proposition~\ref{prop_bigworldignorance2} indicates that there exist some prior beliefs such that all (almost) optimal updating mechanisms will ignore some states. In contrast, Proposition~\ref{prop_bigworldignorance2infiniteN} is ``stronger": for all prior beliefs, all learning mechanisms, including the (almost) optimal updating mechanism, have to be ignorant, and has to ignore almost all states. Roughly speaking, the intuition of Proposition~\ref{prop_bigworldignorance2infiniteN} is as follows: when $M\rightarrow\infty$, the stationary probability of each memory state becomes infinitesimally small. As the DM cannot allocate infinite memory state in almost all $M^{\omega}$, i.e., the DM takes almost all action~$\omega$ in a finite number of memory states, he must choose almost all actions with $0$ probability.

To complete the analysis in the extension, the following corollary shows that disagreement could be persistent in big worlds, as in the baseline model.

\begin{corollary}\label{coro_bigworlddisagreementinfiniteN}
	Fix $N(k)$ and $M(k)$ such that $N(k)=\Theta(M_{i}(k)^{h_{i}})$ with $h_i<1$ for $i=A,B$.  Also assume that $\lim_{N\rightarrow\infty}p^{\omega}_{NA}>0$ if and only if $\lim_{N\rightarrow\infty}p^{\omega}_{NB}>0$ for all $\omega\in\lbrace 1,\cdots\infty\rbrace$. There exists some $\lbrace(\bm{u}^{\omega}_{N(k)i},p^{\omega}_{N(k)i},f^{\omega}_{N(k)i})_{\omega=1}^{N}\rbrace_{k=1}^{\infty}$ where $i=A,B$, such that for all $\epsilon$, there exists some sequences of $\epsilon$-optimal updating mechanism for individual A and B such that they almost always disagree.
\end{corollary}
Note that Corollary~\ref{coro_bigworlddisagreementinfiniteN} is weaker than Corollary~\ref{coro_bigworlddisagreement} in the sense that there exist some, but not all, $\epsilon$-optimal updating mechanisms that lead to disagreement. The intuition is as follows: as shown in Proposition~\ref{prop_bigworldignorance2infiniteN}, the DM must ignore almost all actions. Thus, he obtains positive utility only under a negligible amount of states, and it implies that a large set of updating mechanisms could be $\epsilon$-optimal. In particular, when the prior likelihood of all states are infinitesimally small at the limit, e.g., $p^{\omega}=\frac{1}{N}$, the supremum utility equals $0$ and all updating mechanisms are $\epsilon$-optimal. This leaves ample room for the individuals to adopt different optimal learning mechanisms and thus leads to disagreement. By comparing Corollary~\ref{coro_bigworlddisagreementinfiniteN} and~\ref{coro_agreesmallworld1infiniteN}, we can conclude that the same result in the baseline model holds qualitatively in this extension: asymptotic disagreement does not arise in small worlds but could arise (optimally) in big worlds. 

\section{Example of a sequence of signal structures that satisfies Equation~\ref{assumption_noperfectsignalinfinite} and Assumption~\ref{assumption_identifiableinfinte}}\label{section:signalstructure}

In this section, I provide an example of a sequence of signal structures that satisfies Equation~\ref{assumption_noperfectsignalinfinite} and Assumption~\ref{assumption_identifiableinfinte}. Consider the following seqeunce of signal structures $\lbrace(f_{N}^{\omega})_{\omega=1}^{N}\rbrace_{N=1}^{\infty}$ with $S=[0,1)$:
%\begin{equation*}
%f_{N}^{1}(s)=\begin{cases}
%\frac{2}{3}\text{ for $s\in [\frac{i}{2^{1}},\frac{i+1}{2^{1}})$ where $i=0$}\\
%\frac{4}{3}\text{ for $s\in [\frac{i}{2^{1}},\frac{i+1}{2^{1}})$ where $i=1$}
%\end{cases}
%\end{equation*}
\begin{equation*}
	f_{N}^{\omega}(s)=\begin{cases}
		\frac{2}{3}\text{ for $s\in [\frac{i}{2^{\omega}},\frac{i+1}{2^{\omega}})$ where $i=0,2,\cdots, 2^{\omega}-2$};\\
		\frac{4}{3}\text{ for $s\in [\frac{i}{2^{\omega}},\frac{i+1}{2^{\omega}})$ where $i=1,3,\cdots, 2^{\omega}-1$.}
	\end{cases}
\end{equation*}
The signal structures are illustrated in Figure~\ref{fig:appendixb}. First, they satisfy Equation~\ref{assumption_noperfectsignalinfinite} as $\frac{f_{N}^{\omega}(s)}{f_{N}^{\omega'}(s)}\geq\frac{1}{2}$ for all $\omega,\omega'\in\Omega$, $N$ and $s$. Second,  for any $N$ and given any $\omega$ and $\omega'\neq\omega$, the Cauchy-Schwarz distance is equal to:
\begin{equation*}
	\begin{split}
		-\log\dfrac{\int f_{N}^{\omega}(s)f_{N}^{\omega'}(s)ds}{\sqrt{\int (f_{N}^{\omega}(s))^{2}ds}\sqrt{\int (f_{N}^{\omega'}(s))^{2}ds}}=&-\log\frac{\frac{1}{4}(\frac{2}{3})^{2}+\frac{1}{2}\frac{2}{3}\frac{4}{3}+\frac{1}{4}(\frac{4}{3})^{2}}{\frac{1}{2}(\frac{2}{3})^{2}+\frac{1}{2}(\frac{4}{3})^{2}}\\
		=&-\log\frac{1}{10/9}>1+\xi
	\end{split}
\end{equation*}
where $\xi<\log\frac{10}{9}-1$ and thus satisfies Assumption~\ref{assumption_identifiableinfinte}.

\begin{figure}
	\centering
	\begin{tikzpicture}
		\draw[->] (0,0) node[left] {$\omega=1$} --(10,0) node[right] {$s$};
		\draw (1,0.1)--(1,-0.1) node[below] {$0$};
		\draw (9,0.1)--(9,-0.1) node[below] {$1$};
		\draw (5,0.1)--(5,-0.1) node[below] {$\frac{1}{2}$};
		\node[above] at (3,0.1) {$f^{1}_{N}=\frac{2}{3}$};
		\node[above] at (7,0.1) {$f^{1}_{N}=\frac{4}{3}$};
		\draw[->] (0,-2) node[left] {$\omega=2$} --(10,-2) node[right] {$s$};
		\draw (1,-1.9)--(1,-2.1) node[below] {$0$};
		\draw (9,-1.9)--(9,-2.1) node[below] {$1$};
		\draw (5,-1.9)--(5,-2.1) node[below] {$\frac{2}{2^{2}}$};
		\draw (3,-1.9)--(3,-2.1) node[below] {$\frac{1}{2^{2}}$};
		\draw (7,-1.9)--(7,-2.1) node[below] {$\frac{3}{2^{2}}$};
		\node[above] at (2,-1.9) {$f^{2}_{N}=\frac{2}{3}$};
		\node[above] at (4,-1.9) {$f^{2}_{N}=\frac{4}{3}$};
		\node[above] at (6,-1.9) {$f^{2}_{N}=\frac{2}{3}$};
		\node[above] at (8,-1.9) {$f^{2}_{N}=\frac{4}{3}$};
		\draw[->] (0,-4) node[left] {$\omega=3$} --(10,-4) node[right] {$s$};
		\draw (1,-3.9)--(1,-4.1) node[below] {$0$};
		\draw (9,-3.9)--(9,-4.1) node[below] {$1$};
		\draw (2,-3.9)--(2,-4.1) node[below] {$\frac{1}{2^{3}}$};
		\draw (3,-3.9)--(3,-4.1) node[below] {$\frac{2}{2^{3}}$};
		\draw (4,-3.9)--(4,-4.1) node[below] {$\frac{3}{2^{3}}$};
		\draw (5,-3.9)--(5,-4.1) node[below] {$\frac{4}{2^{3}}$};
		\draw (6,-3.9)--(6,-4.1) node[below] {$\frac{5}{2^{3}}$};
		\draw (7,-3.9)--(7,-4.1) node[below] {$\frac{6}{2^{3}}$};
		\draw (8,-3.9)--(8,-4.1) node[below] {$\frac{7}{2^{3}}$};
		\node[above] at (1.5,-3.9) {\tiny $f^{3}_{N}=\frac{2}{3}$};
		\node[above] at (2.5,-3.9) {\tiny $f^{3}_{N}=\frac{4}{3}$};
		\node[above] at (3.5,-3.9) {\tiny $f^{3}_{N}=\frac{2}{3}$};
		\node[above] at (4.5,-3.9) {\tiny $f^{3}_{N}=\frac{4}{3}$};
		\node[above] at (5.5,-3.9) {\tiny $f^{3}_{N}=\frac{2}{3}$};
		\node[above] at (6.5,-3.9) {\tiny $f^{3}_{N}=\frac{4}{3}$};
		\node[above] at (7.5,-3.9) {\tiny $f^{3}_{N}=\frac{2}{3}$};
		\node[above] at (8.5,-3.9) {\tiny $f^{3}_{N}=\frac{4}{3}$};
		\node at (5,-5.5) {$\vdots$};
	\end{tikzpicture}
	\caption{Signal structures that satisfies Equation~\ref{assumption_noperfectsignalinfinite} and Assumption~\ref{assumption_identifiableinfinte} as $N\rightarrow\infty$. The signal structures comprise low and high density alternatively in $2^{\omega}$ equal-sized intervals.}
	\label{fig:appendixb}
\end{figure}

\section{Robustness of the results in small worlds to updating mistakes}\label{section:robustness}
Below, I show that the behavioral implications is small world, i.e., asymptotic behavior is close to Bayesian, and that disagreement does not persist, hold even when individuals make ``updating mistakes". In other words, the results are robust to individuals' limited ability to design and follow an ``optimal" updating mechanism.

Consider two individuals $A$ and $B$. Individual $A$ adopts the simple updating mechanism described in the proof of Proposition~\ref{prop_smallworld} while individual $B$ ``attempts" to adopt the same updating mechanism but makes local mistakes as he randomly transits to neighboring memory states with some probability $\gamma\in(0,1)$. Formally, the transition rule of individual $B$, denoted as $\mathscr{T}'(m,s)$, is as follows:
\begin{equation*}
	\mathscr{T}'(0,s)=\begin{cases}
		\mathscr{T}(0,s) &\text{ with probability $1-\gamma$;}\\
		ji &\text{ with probability $\frac{\gamma}{N}$ for all $j=1,\cdots,N$.}
	\end{cases}
\end{equation*}
\begin{equation*}
	\mathscr{T}'(i1,s)=\begin{cases}
		\mathscr{T}(i1,s) &\text{ with probability $1-\gamma$;}\\
		i2 &\text{ with probability $\frac{\gamma}{2}$;}\\
		0&\text{ with probability $\frac{\gamma}{2}$.}
	\end{cases}
\end{equation*}
\begin{equation*}
	\mathscr{T}'(i\lambda,s)=
	\begin{cases}
		\mathscr{T}(i\lambda,s)&\text{ with probability $1-\gamma$;}\\
		i(\lambda-1) &\text{ with probability $\gamma$.}
	\end{cases}
\end{equation*}
while for $k=2,3,\cdots,\lambda-1$,
\begin{equation*}
	\mathscr{T}'(ik,s)=\begin{cases}
		\mathscr{T}(ik,s) &\text{ with probability $1-\gamma$;}\\
		i(k-1) &\text{ with probability $\frac{\gamma}{2}$;}\\
		i(k+1)&\text{ with probability $\frac{\gamma}{2}$.}
	\end{cases}
\end{equation*}
where $\mathscr{T}(m,s)$ is defined in the proof of Proposition~\ref{prop_smallworld}. The initial memory states and decision rule of individual B stay the same as individual A. Such updating mistakes could be induced by memory imperfections, i.e., the DM's memory state is subject to local fluctuations, or imperfect perceptions on signals, e.g., the DM may mistakenly perceive any signal as a signal that supports state~$\omega$. 

\begin{proposition}\label{prop_smallworldmistakes}
	Consider individual $A$ who adopts the updating mechanism $\mathscr{T}$ and individual $B$ who makes local mistakes with some probability $\gamma\in(0,1)$, characterized above by $\mathscr{T}'(m,s)$. Fix $N$ and $(\bm{u}_B^{\omega}, p_B^{\omega}, f_B^{\omega})_{\omega=1}^{N}$, for all $\gamma\in(0,1)$,
	\begin{equation*}
		\lim_{k\rightarrow\infty} L_k(m_1,\mathscr{T}',d)=0.
	\end{equation*}
	Moreover, individual $A$ and $B$ are bound to agree in small worlds. %, i.e., for all $(\bm{u}^{\omega}_{A},p^{\omega}_{A},f^{\omega}_{A})_{\omega=1}^{N}$, $(\bm{u}^{\omega}_{B},p^{\omega}_{B},f^{\omega}_{B})_{\omega=1}^{N}$, fixing $N$ and $M\rightarrow\infty$,
	%\begin{equation*}
		%\lim_{T\rightarrow\infty}E_{\omega,\mathscr{T},\mathscr{T}'}\left[\frac{\sum_{t=1}^T\mathbbm{1}_{a_t^A= a_t^B}}{T}\right]=0 \text{ for all $\omega$}.
	%\end{equation*}
\end{proposition}

\section{Proof of the results in online appendix}
\subsection{Proof of Proposition~\ref{prop_discountfactor}}
\begin{proof}
	Suppose to the contrary that $\lim_{\rho\rightarrow 1}L(m^{*D}_1(\rho),\mathscr{T}^{*D}(\rho),d^{*D}(\rho))>L^*_M+\epsilon$ for some $\epsilon>0$. It implies that there exists some updating mechanism $(m_1,\mathscr{T},d)$ that yields strictly higher asymptotic utility than $(m^{*D}_1(\rho),\mathscr{T}^{*D}(\rho),d^{*D}(\rho))$ for all $\rho$ close to 1. By continuity, $(m_1,\mathscr{T},d)$ also yields strictly higher discounted sum of utility than $(m^{*D}_1(\rho),\mathscr{T}^{*D}(\rho),d^{*D}(\rho))$ for all $\rho$ close to $1$. The result follows by contradiction.
\end{proof}

\subsection{Proof of Proposition~\ref{prop_smallworldinfiniteN}}
\begin{proof}
	I show that for all $\epsilon>0$, there exists a sequence of updating mechanisms with utility losses that converge to smaller than $\epsilon$ as $k\rightarrow\infty$. First, by Assumption~\ref{assumption_identifiableinfinte}, for all $\frac{\epsilon}{\bar{u}}>0$, there exists an $\xi>0$ and a sequence of subset of states $N_{\xi}$ such that $\lim_{N\rightarrow\infty}\left(\sum_{\omega\in N_{\xi}}p_{N}^{\omega}\right)>1-\frac{\epsilon}{\bar{u}}$ and
	\begin{equation*}
		\lim_{N\rightarrow\infty}\inf_{\omega,\omega'\in N_{\xi}; \omega'\neq\omega}\left\lbrace-\log\dfrac{\int f_{N}^{\omega}(s)f_{N}^{\omega'}(s)ds}{\sqrt{\int (f_{N}^{\omega}(s))^{2}ds}\sqrt{\int (f_{N}^{\omega'}(s))^{2}ds}}\right\rbrace>\xi
	\end{equation*}
	Before proving the Proposition, I first prove the following Lemma for $(G_{N}^{\omega}(s))_{\omega=1}^{N}$ defined as:
		\begin{equation*}
		G^{\omega}_{N}(s)=\dfrac{f^{\omega}_{N}(s)}{\sqrt{\int (f^{\omega}_{N}(s))^{2}ds}}.
	\end{equation*}
	\begin{lemma}\label{lemmasmallworldinfoinfiniteas}
		For $\frac{\epsilon}{\bar{u}}>0$, there exists an $\tilde{\xi}>0$, a sequence of $\delta_{N}>1$ and a sequence of subset of states $N_{\xi}$ with $\lim_{N\rightarrow\infty}\left(\sum_{\omega\in N_{\xi}}p_{N}^{\omega}\right)>1-\frac{\epsilon}{\bar{u}}$ such that
		\begin{equation}\label{eq:smallworldinfinite}
			\begin{split}
				\frac{\delta_{N}F_{N}^{\omega}(G_{N}^{\omega'})}{\sum_{\omega''\neq\omega'}F_{N}^{\omega}(G_{N}^{\omega''})} > 2\text{ for all $\omega,\omega'\in\Omega$ and $N$;}&\\
				%\lim_{N,M\rightarrow\infty}\frac{\delta_{N}F^{\omega}(S_{\omega'})}{\sum_{\omega''\neq\omega'}F^{\omega}(S_{\omega''})}=\infty \text{ for all $\omega,\omega'\in\Omega$;}&\\
				\lim_{N\rightarrow\infty}\inf_{\omega,\omega'\in N_{\xi}; \omega'\neq\omega}\dfrac{\dfrac{\delta_{N} F_{N}^{\omega}(G_{N}^{\omega})}{\sum_{\omega''\neq\omega}F_{N}^{\omega}(G_{N}^{\omega''})}}{\dfrac{\delta_{N} F_{N}^{\omega}(G_{N}^{\omega'})}{\sum_{\omega''\neq\omega'} F_{N}^{\omega}(G_{N}^{\omega''})}}>1+\tilde{\xi}.&
			\end{split}
		\end{equation}
	\end{lemma}
	\begin{proof}
		As $F_{N}^{\omega}(G_{N}^{\omega'})>0$ for all $\omega,\omega'$, there always exists a big enough $\delta_{N}$ such that the first inequality of Equation~\eqref{eq:smallworldinfinite} holds. To prove the second Inequality, note that
		\begin{align}\label{eq:smallworldinfinitelemma}
				\allowdisplaybreaks\nonumber&\lim_{N\rightarrow\infty}\inf_{\omega,\omega'\in N_{\xi}; \omega'\neq\omega}\dfrac{\dfrac{\delta_{N} F_{N}^{\omega}(G_{N}^{\omega})}{\sum_{\omega''\neq\omega}F_{N}^{\omega}(G_{N}^{\omega''})}}{\dfrac{\delta_{N} F_{N}^{\omega}(G_{N}^{\omega'})}{\sum_{\omega''\neq\omega'} F_{N}^{\omega}(G_{N}^{\omega''})}}\\\allowdisplaybreaks
				\geq&\lim_{N\rightarrow\infty}\inf_{\omega,\omega'\in N_{\xi}; \omega'\neq\omega}\dfrac{F_{N}^{\omega}(G_{N}^{\omega})}{F_{N}^{\omega}(G_{N}^{\omega'})}\\\nonumber\allowdisplaybreaks
				=&\lim_{N\rightarrow\infty}\inf_{\omega,\omega'\in N_{\xi}; \omega'\neq\omega}\dfrac{\sqrt{\int (f_{N}^{\omega}(s))^{2}ds}\sqrt{\int (f_{N}^{\omega'}(s))^{2}ds}}{\int f_{N}^{\omega}(s)f_{N}^{\omega'}(s)ds}\\\nonumber
				>&\exp{(\xi)}\\\nonumber\allowdisplaybreaks
				=&1+\tilde{\xi}\nonumber\allowdisplaybreaks
		\end{align}	
		where $\tilde{\xi}=1-\exp{(\xi)}$ and the first inequality of Equation~\eqref{eq:smallworldinfinitelemma} is implied by the fact that $F_{N}^{\omega}(G_{N}^{\omega})\geq F_{N}^{\omega}(G_{N}^{\omega'})$ and thus $\frac{\sum_{\omega''\neq\omega'} F_{N}^{\omega}(G_{N}^{\omega''})}{\sum_{\omega''\neq\omega} F_{N}^{\omega}(G_{N}^{\omega''})}\geq 1$.
	\end{proof}
	Now consider a sequence of updating mechanisms described in the proof of Proposition~\ref{prop_smallworld}, but include only states in $N_{\xi}$, i.e., there are only branches that correspond to actions in $N_{\xi}$,  and there exists no $m\in M$ such that $d(m)=\omega'$ for $\omega'\notin N_{\xi}$. As in the proof of Proposition~\ref{prop_smallworld}, denote $\frac{\delta_{N} F_{N}^{\omega}(G_{N}^{\omega'})}{\sum_{\omega''\neq\omega'}F_{N}^{\omega}(G_{N}^{\omega''})}$ as $r^{\omega\omega'}_{N}$, the stationary distribution under state $\omega\in N_{\xi}$ is as follows:
	\begin{equation}
		%\lim_{N,M\rightarrow\infty}\Biggl\lbrace
		\mu^{\omega}_{N\omega\lambda}\sum_{i=1}^{\lambda}\left[r^{\omega\omega}_{N}\right]^{-(\lambda-i)}+\mu^{\omega}_{N\omega\lambda}\left[r^{\omega\omega}_{N}\right]^{-\lambda}
		+\mu^{\omega}_{N\omega\lambda}\left[r^{\omega\omega}_{N}\right]^{-\lambda}\sum_{\omega'\in N_{\xi}\setminus\lbrace\omega\rbrace}\sum_{i=1}^{\lambda}\left[r^{\omega\omega'}_{N}\right]^{(\lambda-i)}%\Biggr\rbrace
		=1
	\end{equation}
	where $\mu^{\omega}_{Nm}$ is the stationary probability in memory state $m$ under state $\omega$ when state space has size $N$. %First note that $\lim_{k\rightarrow\infty}\frac{M(k)}{N(k)}=\lim_{k\rightarrow\infty}\lambda(k)=\infty$.
	 Given the first inequality of Lemma~\ref{lemmasmallworldinfoinfiniteas}, $r^{\omega\omega}_{N}>2$ for all $\omega$ and $N$ and therefore $\lim_{k\rightarrow\infty}\mu^{\omega}_{N(k)\omega\lambda}\left[r^{\omega\omega}_{N(k)}\right]^{-\lambda(k)}=0$. On the other hand,
	\begin{align*}
			\left[r^{\omega\omega}_{N}\right]^{-\lambda}\sum_{\omega'\in N_{\xi}\setminus\lbrace\omega\rbrace}\sum_{i=1}^{\lambda}\left[r^{\omega\omega'}_{N}\right]^{(\lambda-i)}
			=&\left[r^{\omega\omega}_{N}\right]^{-\lambda}\sum_{\omega'\in N_{\xi}\setminus\lbrace\omega\rbrace}\frac{\left[r^{\omega\omega'}_{N}\right]^{\lambda}-1}{r^{\omega\omega'}_{N}-1}\\
			\leq&\sum_{\omega'\in N_{\xi}\setminus\lbrace\omega\rbrace}\left[\left[\frac{r^{\omega\omega'}_{N}}{r^{\omega\omega}_{N}}\right]^{\lambda}-\left[r^{\omega\omega'}_{N}\right]^{-\lambda}\right]\\
			\leq&\sum_{\omega'\in N_{\xi}\setminus\lbrace\omega\rbrace}(1+\tilde{\xi})^{-\lambda}
			\leq N(1+\tilde{\xi})^{-\lambda}
	\end{align*}
	where the first inequality is implied by the first inequality in Lemma~\ref{lemmasmallworldinfoinfiniteas}, and the second inequality is implied by the second inequality in Lemma~\ref{lemmasmallworldinfoinfiniteas} and that $\left[r^{\omega\omega'}_{N}\right]^{-\lambda}>0$. As $(1+\tilde{\xi})^{-\lambda}$ converges to $0$ exponentially and $N$ converges to infinity linearly, $\lim_{k\rightarrow\infty}N(k)(1+\tilde{\xi})^{-\lambda(k)}=0$. To see it formally, note that $N(k)=\Theta(M(k)^{h})$ with $h<1$ and $\lambda(k)=\frac{M(k)}{N(k)}$ imply that $\lambda(k)=\Theta(M(k)^{1-h})$. By the definition of $\Theta$, we have for some constant $K$ and some $q$ big enough such that
	\begin{equation*}
		\begin{split}
			\frac{N(k)}{(1+\tilde{\xi})^{\lambda(k)}}\leq K\frac{M(k)^{h}}{(1+\tilde{\xi})^{M(k)(1-h)}}&=K\left[\frac{M(k)}{(1+\tilde{\xi})^{M(k)\frac{1-h}{h}}}\right]^{h}\\
			&=K\left[\frac{M(k)}{(1+\tilde{\tilde{\xi}})^{M(k)}}\right]^{h}\\
			&<K\left[\frac{M(k)}{{M(k)\choose 2}\tilde{\tilde{\xi}}^2}\right]^{h}\\
			&=K\left[\frac{2}{(M(k)-1)\tilde{\tilde{\xi}}^2}\right]^{h}
		\end{split}
	\end{equation*}
	where $1+\tilde{\tilde{\xi}}=(1+\tilde{\xi})^{\frac{1-h}{h}}$ and the second inequality is implied by the Binomial Theorem. Thus,
	\begin{equation*}
		\begin{split}
				\lim_{k\rightarrow\infty}\left[r^{\omega\omega}_{N}\right]^{-\lambda}\sum_{\omega'\in N_{\xi}\setminus\lbrace\omega\rbrace}\sum_{i=1}^{\lambda}\left[r^{\omega\omega'}_{N}\right]^{(\lambda-i)}\leq&\lim_{k\rightarrow\infty}\left[r^{\omega\omega}_{N}\right]^{-\lambda}N(1+\tilde{\xi})^{-\lambda(k)}\\
				<&\lim_{k\rightarrow\infty}\left[r^{\omega\omega}_{N}\right]^{-\lambda}K\left[\frac{2}{(M(k)-1)\tilde{\tilde{\xi}}^2}\right]^{h}=0.
		\end{split}
	\end{equation*}
	It implies that $\lim_{k\rightarrow\infty}\left[r^{\omega\omega}_{N}\right]^{-\lambda}\sum_{\omega'\in N_{\xi}\setminus\lbrace\omega\rbrace}\sum_{i=1}^{\lambda}\left[r^{\omega\omega'}_{N}\right]^{(\lambda-i)}=0$ and
	\begin{equation}
		\lim_{k\rightarrow\infty}\sum_{i=1}^{\lambda}\mu^{\omega}_{N\omega i}=\lim_{k\rightarrow\infty}\mu^{\mu}_{N\omega\lambda}\sum_{i=1}^{\lambda}\left[r^{\omega\omega}_{N}\right]^{-(\lambda-i)}=1
	\end{equation}
	for all $\omega\in N_{\xi}$. In state $\omega\in N_{\xi}$, the DM chooses action~$\omega$ with asymptotic probability equal to $1$. As $\lim_{N\rightarrow\infty}\sum_{\omega\in N_{\xi}}p_{N}^{\omega}>1-\frac{\epsilon}{\bar{u}}$, the asymptotic utility loss of the proposed non-ignorant updating mechanism is strictly bounded above by $\bar{u}\times\frac{\epsilon}{\bar{u}}=\epsilon$.
\end{proof}

\subsection{Proof of Corollary~\ref{coro_ignorancesmallworldinfinteN}}
\begin{proof}
	Suppose in contrary the sequence of updating mechanisms ignore strictly more than $\frac{\epsilon}{\underline{u}}$ measures of states at the limit. That is, denoted $\tilde{N}(k)$ as the set of states that is ignored for a given sequence of updating mechanism at the limit, we have $\lim_{T\rightarrow\infty}E_{\omega'}\left[\frac{\sum_{t=1}^{T}\mathbbm{1}_{a_t\in \tilde{N}(k)}}{T}\right]=0$ for (almost) all $\omega'$ and  $\lim_{k\rightarrow\infty}\sum_{\omega\in\tilde{N}(k)}p^{\omega}_{N(k)}>\frac{\epsilon}{\underline{u}}$. The utility loss as $k\rightarrow \infty$ is
	\begin{multline*}
		\lim_{k\rightarrow \infty} L_{k}\geq\lim_{k\rightarrow\infty}\sum_{\omega\in\tilde{N}(k)}\left[u_{N(k)}(\omega,\omega)-\max_{\omega'\neq\omega}u(\omega',\omega)\right]p_{N(k)}^{\omega}\\\geq\underline{u}\lim_{k\rightarrow\infty}\sum_{\omega\in\tilde{N}(k)}p_{N(k)}^{\omega}>\underline{u}\frac{\epsilon}{\underline{u}}=\epsilon=\lim_{k\rightarrow \infty}L_{k}^{*}+\epsilon
	\end{multline*}
	which proves the result.
\end{proof}

\subsection{Proof of Corollary~\ref{coro_agreesmallworld1infiniteN}}
\begin{proof}
	With some abuse of notation, denote $\pmb{\mathscr{T}^{\epsilon}_{ki}}$ as the set of $\epsilon$-optimal updating mechanism of individual $i=A,B$. By Proposition~\ref{prop_smallworldinfiniteN}, we have:
	\begin{equation*}
		\lim_{k\rightarrow\infty}\lim_{\epsilon\rightarrow 0}\sup_{(m_{1ki},\mathscr{T}_{ki},d_{ki})\in\pmb{\mathscr{T}^{\epsilon}_{ki}}}\sum_{\omega}\left[\mathbbm{1}\left\lbrace\lim_{T\rightarrow \infty}E_{\omega,\mathscr{T}_{ki}}\frac{\sum_{t=1}^{T}\mathbbm{1}_{a^i_t=\omega}}{T}=1\right\rbrace p^{\omega}_{Ni}\right]=1
	\end{equation*}
	which is equivalent to
	\begin{equation*}
		\lim_{k\rightarrow\infty}\lim_{\epsilon\rightarrow 0}\sup_{(m_{1ki},\mathscr{T}_{ki},d_{ki})\in\pmb{\mathscr{T}^{\epsilon}_{ki}}}\sum_{\omega}\left[\mathbbm{1}\left\lbrace\lim_{T\rightarrow \infty}E_{\omega,\mathscr{T}_{ki}}\frac{\sum_{t=1}^{T}\mathbbm{1}_{a^i_t=\omega}}{T}<1\right\rbrace p^{\omega}_{Ni}\right]=0,
	\end{equation*}
	i.e., individual $i$ would only take sub-optimal actions in probability $0$ events measured by $(p_{Ni}^{\omega})_{\omega=1}^{N}$. As $\lim_{N\rightarrow\infty}p^{\omega}_{NA}>0$ if and only if $\lim_{N\rightarrow\infty}p^{\omega}_{NB}>0$ for all $\omega$, combined with Assumption~\ref{assumption_fullsupportinfinite}, this implies that 
	\begin{equation*}
		\lim_{k\rightarrow\infty}\sum_{\omega\in \tilde{\Omega}(k)} p^{\omega}_{NA}=0 \text{ if and only if  }\lim_{k\rightarrow\infty}\sum_{\omega\in \tilde{\Omega}(k)} p^{\omega}_{NB}=0
	\end{equation*}
	for all $\tilde{\Omega}(k)\in\lbrace1,\cdots,N(k)\rbrace$. Thus, 
		\begin{equation*}
		\lim_{k\rightarrow\infty}\lim_{\epsilon\rightarrow 0}\sup_{(m_{1ki},\mathscr{T}_{ki},d_{ki})\in\pmb{\mathscr{T}^{\epsilon}_{ki}}}\sum_{\omega}\left[\mathbbm{1}\left\lbrace\lim_{T\rightarrow \infty}E_{\omega,\mathscr{T}_{ki}}\frac{\sum_{t=1}^{T}\mathbbm{1}_{a^i_t=\omega}}{T}<1\right\rbrace p^{\omega}_{NI}\right]=0\text{ for all $i,I\in\lbrace A,B\rbrace$}
	\end{equation*}
	and
	\begin{equation*}
		\begin{split}
			&\lim_{k\rightarrow\infty}\lim_{\epsilon\rightarrow 0}\sup_{(m_{1kA},\mathscr{T}_{kA},d_{kA})\in\pmb{\mathscr{T}^{\epsilon}_{kA}},(m_{1kB},\mathscr{T}_{kB},d_{kB})\in\pmb{\mathscr{T}^{\epsilon}_{kB}}}\sum_{\omega}\left[\mathbbm{1}\left\lbrace\lim_{T\rightarrow \infty}E_{\omega,\mathscr{T}_{kA},\mathscr{T}_{kB}}\frac{\sum_{t=1}^{T}\mathbbm{1}_{a^A_t=a^{B}_t=\omega}}{T}<1\right\rbrace p^{\omega}_{Ni}\right]\\
			\leq &\lim_{k\rightarrow\infty}\lim_{\epsilon\rightarrow 0}\sup_{(m_{1kA},\mathscr{T}_{kA},d_{kA})\in\pmb{\mathscr{T}^{\epsilon}_{kA}}}\sum_{\omega}\left[\mathbbm{1}\left\lbrace\lim_{T\rightarrow \infty}E_{\omega,\mathscr{T}_{kA}}\frac{\sum_{t=1}^{T}\mathbbm{1}_{a^A_t=\omega}}{T}<1\right\rbrace p^{\omega}_{Ni}\right]\\
			&+\lim_{k\rightarrow\infty}\lim_{\epsilon\rightarrow 0}\sup_{(m_{1kB},\mathscr{T}_{kB},d_{kB})\in\pmb{\mathscr{T}^{\epsilon}_{kB}}}\sum_{\omega}\left[\mathbbm{1}\left\lbrace\lim_{T\rightarrow \infty}E_{\omega,\mathscr{T}_{kB}}\frac{\sum_{t=1}^{T}\mathbbm{1}_{a^B_t=\omega}}{T}<1\right\rbrace p^{\omega}_{Ni}\right]\\
			=&0
		\end{split}
	\end{equation*}
	for $i=A,B$. The result follows.
\end{proof}

\subsection{Proof of Proposition~\ref{prop_bayesianlearningbigworldinfiniteN}}
\begin{proof}
	First, note that for $\lim_{k\rightarrow \infty}L_{k}^{*}=0$, denote $M_k^{\omega}=\lbrace m: d_k(m)=\omega\rbrace$, we must have for some $\lbrace m_{1k},\mathscr{T}_k,d_k\rbrace_{k=1}^{\infty}$,
	\begin{equation*}
		\lim_{k\rightarrow \infty}\sum_{m\in M_k^{\omega}}\mu_{N(k)m}^{\omega}=1
	\end{equation*}
	for almost all $\omega$, i.e., there must exist a sequence of subsets of states $\hat{\Omega}(k)\in\lbrace1,\cdots,N(k)\rbrace$ where $\lim_{k\rightarrow\infty}\sum_{\omega\in\hat{\Omega}(k)}p_{N(k)}^{\omega}=1$ and 
	\begin{equation*}
		\lim_{k\rightarrow \infty}\sum_{m\in M_k^{\omega}}\mu_{N(k)m}^{\omega}=1.
	\end{equation*}
	for all $\omega\in\hat{\Omega}(k)$. Additionally, Assumption~\ref{assumption_fullsupportinfinite} implies that there must exist a sequence of subsets of states $\hat{\Omega}(k)\in\lbrace1,\cdots,N(k)\rbrace$ where $\lim_{k\rightarrow}\frac{\vert\hat{\Omega}(k)\vert}{N(k)}=1$ and 
	\begin{equation*}
		\lim_{k\rightarrow \infty}\sum_{m\in M_k^{\omega}}\mu_{N(k)m}^{\omega}=1,
	\end{equation*}
	for all $\omega\in\hat{\Omega}(k)$. That is, the DM chooses the optimal action in almost all states, measured in both prior probability or in fraction. It implies that for all $\omega$ in $\hat{\Omega}(k)$, there must exist a set of memory state $\hat{M}_k^{\omega}\subseteq M_k^{\omega}$ such that 
	\begin{equation}
		\begin{split}
			\lim_{k\rightarrow\infty}\sum_{m\in\hat{M}_{k}^{\omega}}\mu^{\omega}_{N(k)m}&=1;\\
			\lim_{k\rightarrow\infty}\sum_{m\in\hat{M}_{k}^{\omega}}\mu^{\omega'}_{N(k)m}&=0\text{ for all $\omega'\in\hat{\Omega}(k)\setminus\lbrace\omega\rbrace$;}\\
			\lim_{k\rightarrow\infty}\max_{m\in\hat{M}_{k}^{\omega}}\frac{\mu_{N(k)m}^{\omega}}{\mu_{N(k)m}^{\omega'}}&=\infty\text{ for all $\omega'\in\hat{\Omega}(k)\setminus\lbrace\omega\rbrace$}.\\
		\end{split}
		\label{eq:bigworldfirstequation}
	\end{equation}
	In the following I prove that for Equation~\eqref{eq:bigworldfirstequation} to hold, $\frac{M}{N}$ has to go to $\infty$. First consider an irreducible automaton $\mathscr{T}_{k}$. Fix a $\omega'\in\hat{\Omega}(k)\setminus\lbrace\omega\rbrace$, without loss of generality rearrange the memory states such that $\frac{\mu^{\omega}_{N(k)m}}{\mu^{\omega'}_{N(k)m}}$ is weakly decreasing in $m$. As argued in the proof of Proposition~\ref{prop_bigworldignorance2}, Lemma 2 of \cite{hellman1970learning} holds in the current setting, so that for all $m<M(k)$,
	\begin{equation}
		\begin{split}
			\frac{\mu^{\omega}_{N(m+1)}}{\mu^{\omega'}_{N(m+1)}}&\geq (\overline{l}_{N}^{\omega\omega'}\overline{l}_{N}^{\omega'\omega})^{-1}\frac{\mu^{\omega}_{Nm}}{\mu^{\omega'}_{Nm}}\\
			&\geq\varsigma^{2}\frac{\mu^{\omega}_{Nm}}{\mu^{\omega'}_{Nm}}.
		\end{split}
		\label{eq:bigworldsecondequation}
	\end{equation}
	in which I omitted the argument in $N(k)$ for ease of exposition. If $\max_{m}\frac{\mu^{\omega}_{Nm}}{\mu^{\omega'}_{Nm}}=\frac{\mu^{\omega}_{N1}}{\mu^{\omega'}_{N1}}>K$, Equation~\eqref{eq:bigworldsecondequation} implies that 
	\begin{equation*}
		\frac{\mu^{\omega}_{Nm'}}{\mu^{\omega'}_{Nm'}}\geq\varsigma^{2(m'-1)}\frac{\mu^{\omega}_{N1}}{\mu^{\omega'}_{N1}}>\varsigma^{2(m'-1)}K.
	\end{equation*}
	As there must exist some $m'$ with $\frac{\mu^{\omega}_{Nm'}}{\mu^{\omega'}_{Nm'}}\leq 1$, there must exist at least $\frac{\log K}{-2\log \varsigma}+1$ memory states with $\frac{\mu^{\omega}_{Nm}}{\mu^{\omega'}_{Nm}}\geq 1$. Repeating the same analysis for other $\omega''\in \hat{\Omega}(k)\setminus\lbrace\omega\rbrace$ implies that if $\max_m\frac{\mu^{\omega}_{Nm}}{\mu^{\omega''}_{Nm}}>K$ for all $\omega''\in \hat{\Omega}(k)\setminus\lbrace\omega'\rbrace$, there must exist at $\frac{\log K}{-2\log \varsigma}+1$ memory states with a likelihood ratio $\min_{\omega'\in\hat{\Omega}(k)}\frac{\mu_{Nm}^{\omega}}{\mu_{Nm}^{\omega'}}\geq 1$. 
	
	With the same argument, if $\max_{m}\frac{\mu^{\omega}_{Nm}}{\mu^{\omega'}_{Nm}}>K$ for all $\omega\in\hat{\Omega}(k)$ and all $\omega'\in\hat{\Omega}(k)\setminus\lbrace\omega\rbrace$, 
		there must exists $\frac{\log K}{-2\log \varsigma}+1$ memory states with a likelihood ratio $\min_{\omega'\in\hat{\Omega}(k)}\frac{\mu_{Nm}^{\omega}}{\mu_{Nm}^{\omega'}}\geq 1$ for all $\omega\in\hat{\Omega}(k)$. Therefore, $\frac{M}{\vert\hat{\Omega}(k)\vert}\geq \frac{\log K}{-2\log \varsigma}+1$. This implies that $\frac{M}{\vert \hat{N}\vert}$ goes to $\infty$ as $K$ goes to $\infty$, which contradicts the fact that $\lim_{k\rightarrow\infty}\frac{M(N)}{\vert \hat{\Omega}(k)\vert}=\lim_{k\rightarrow\infty}\frac{M(k)}{N(k)}<\infty$ in big worlds.
	
	Now I analysis the case of reducible automatons. Denote the recurrent communicating classes as $\mathscr{R}_{k1},\cdots,\mathscr{R}_{kr}$, and the set of transient memory states as $\mathscr{R}_{k0}$. The analysis above applies in the cases where there is only one recurrent communicating class or where the initial memory state is in one of the recurrent communicating classes. 
	
	Now consider the case where $r>1$, i.e., there are more than one recurrent communicating class, and the initial memory state denoted by $i$ is in $\mathscr{R}_{k0}$. I first compute the probability of absorption by $\mathscr{R}_{kj}$ under state $\omega$, denoted by $\mathscr{P}_{k}^{\omega}(\mathscr{R}_{kj})$. Consider a new transition rule $\mathscr{T}'_k$ where all transitions from $m\in\mathscr{R}_{k0}$ to another $m'\in\mathscr{R}_{k0}$ are the same as before. However, $\mathscr{T}'_k$ differs from $\mathscr{T}_k$ that all transitions from $m\in\mathscr{R}_{k0}$ to $m'\notin\mathscr{R}_{k0}$ are changed to transition from $m$ to $i$. Given such a transition rule $\mathscr{T}'_k$, obviously only memory states in $\mathscr{R}_{k0}$ are reachable. Denote $\mu^{0\omega}_{Nm}$ as the stationary distribution of this new transition rule $\mathscr{T}'_k$.
	
	As is known in the theory of Markov chain (see Appendix 2 of \cite{hellman1969learning}), $\mathscr{P}_{k}^{\omega}(\mathscr{R}_{kj})$ is given by:
	\begin{equation*}
		\mathscr{P}_{k}^{\omega}(\mathscr{R}_{kj})=\sum_{m\in\mathscr{R}_{k0}}\mu^{0\omega}_{Nm}\sum_{m'\in\mathscr{R}_{kj}}q^{\omega}_{mm'}
	\end{equation*}
	Also denote $\mu_{Nm}^{j\omega}$ as the stationary distribution within the recurrent communicating class $\mathscr{R}_{kj}$ given $\mathscr{T}_k$, i.e., $\mu_{Nm}^{j\omega}=\frac{\mu_{Nm}^{\omega}}{\sum_{m\in\mathscr{R}_{kj}}\mu_{Nm}^{\omega}}$, we have for $m\in\mathscr{R}_{kj}$
	\begin{equation*}
		\begin{split}
			\frac{\mu^{\omega}_{Nm}}{\mu^{\omega'}_{Nm}}=&\frac{\mathscr{P}_{k}^{\omega}(\mathscr{R}_{kj})}{\mathscr{P}_{k}^{\omega'}(\mathscr{R}_{kj})}\times \frac{\mu^{j\omega}_{Nm}}{\mu^{j\omega'}_{Nm}}\\
			=&\frac{\sum_{m\in\mathscr{R}_{k0}}\mu^{0\omega}_{Nm}\sum_{m'\in\mathscr{R}_{kj}}q^{\omega}_{mm'}}{\sum_{m\in\mathscr{R}_{k0}}\mu^{0\omega'}_{Nm}\sum_{m'\in\mathscr{R}_{kj}}q^{\omega'}_{mm'}}\times \frac{\mu^{j\omega}_{Nm}}{\mu^{j\omega'}_{Nm}}\\
			\leq& \varsigma^{-2}\frac{\sum_{m\in\mathscr{R}_{k0}}\mu^{0\omega}_{Nm}}{\sum_{m\in\mathscr{R}_{k0}}\mu^{0\omega'}_{Nm}}\times \frac{\mu^{j\omega}_{Nm}}{\mu^{j\omega'}_{Nm}}\\
			\leq& \varsigma^{-2}\max_{m\in\mathscr{R}_{k0}}\frac{\mu^{0\omega}_{Nm}}{\mu^{0\omega}_{Nm}}\times \frac{\mu^{j\omega}_{Nm}}{\mu^{j\omega'}_{Nm}}.
		\end{split}
	\end{equation*}
	Thus, if $\max_m \frac{\mu^{\omega}_{Nm}}{\mu^{\omega'}_{Nm}}>K$, we must have 
	\begin{equation*}
		\varsigma^{-2}\max_{m\in\mathscr{R}_{0}}\frac{\mu^{0\omega}_{Nm}}{\mu^{0\omega}_{Nm}}\times \max_{j\in\lbrace 1,2,\cdots, r\rbrace}\max_{m\in\mathscr{R}_{j}}\frac{\mu^{j\omega}_{Nm}}{\mu^{j\omega'}_{Nm}}>K
	\end{equation*}
	Thus, we must have either
	\begin{equation*}
		\begin{split}
			\max_{m\in\mathscr{R}_{0}}\frac{\mu^{0\omega}_{Nm}}{\mu^{0\omega}_{Nm}}&>\varsigma\sqrt{K}\text{, or;}\\
			\max_{j\in\lbrace 1,2,\cdots, r\rbrace}\max_{m\in\mathscr{R}_{j}}\frac{\mu^{j\omega}_{Nm}}{\mu^{j\omega'}_{Nm}}&>\varsigma\sqrt{K}.
		\end{split}
	\end{equation*}
	Then the result follows similar arguments in the case of irreducible automatons.
\end{proof}

\subsection{Proof of Proposition~\ref{prop_bigworldignorance2infiniteN}}
\begin{proof}
	Suppose to the contrary that there exists a sequence of subsets of states $\tilde{\Omega}_{k}$ where $\lim_{k\rightarrow\infty}\frac{\vert\tilde{\Omega}_{k}\vert}{N(k)}>0$, and that for all $\omega\in\tilde{\Omega}_{k}$, the DM takes action~$\omega$ with some strictly positive probability in some state $\omega'\in \lbrace 1,\cdots, N(k)\rbrace$ at the limit where $k\rightarrow\infty$ (where $\omega'$ could be different for different $\omega$). Formally, this implies that for all $\omega\in\tilde{\Omega}_{k}$
	\begin{equation*}
		\lim_{k\rightarrow\infty}\sum_{m\in M^{\omega}_{k}}\mu^{\omega'}_{km}\geq\xi
	\end{equation*}
	for some $\omega'$ and $\xi>0$. As $M_k^{\omega}$ must be finite for almost all $\omega$ (measured in fraction), it implies that there exists some $\tilde{\Omega'}_{k}$ where $\lim_{k\rightarrow\infty}\frac{\vert\tilde{\Omega'}_{k}\vert}{N(k)}>0$, and that for all $\omega\in\tilde{\Omega'}_{k}$ there exists some $\omega'\in\lbrace 1,\cdots, N(k)\rbrace$,
	\begin{equation*}
		\lim_{k\rightarrow\infty}\mu^{\omega'}_{km}\geq\xi'>0 \text{ for some $m\in M^{\omega}_{k}$}.
	\end{equation*}
	
	Now denote the set of $\omega'$, that is, the set of states of the world where the DM picks some action $\omega\in\tilde{\Omega'}_{k}$ with strictly positive probability, as $\tilde{\Omega}''_{k}$. First, we must have $\lim_{k\rightarrow\infty}\frac{\vert\tilde{\Omega'}''_{k}\vert}{N(k)}>0$. Otherwise, there must exist some $\omega'\in\tilde{\Omega}''_{k}$ such that there are infinitely many memory states with probability bigger than $\xi'$ which contradicts the fact that $\lim_{k\rightarrow\infty}\sum_{m=1}^{M}\mu^{\omega'}_{km}=1$. With similar arguments, for almost all $\omega\in\tilde{\Omega'}_{k}$, there must exist some $m\in M^{\omega}_k$ such that $\lim_{k\rightarrow\infty}\mu^{\omega'}_{km}\geq\xi'$ for some $\omega'\in\tilde{\Omega}''_{k}$ but $\lim_{k\rightarrow\infty}\mu^{\omega''}_{km}=0$ for almost all (measured in fraction) states $\omega''\in\tilde{\Omega'}_{k}\setminus\lbrace\omega'\rbrace$. This implies that there exists some sequence of subsets of states $\tilde{\tilde{\Omega_k}}$ where $\lim_{N\rightarrow\infty}\frac{\vert\tilde{\tilde{\Omega_k}}\vert}{N}>0$ such that
	\begin{equation*}
		\lim_{k\rightarrow\infty}\max_{m}\frac{\mu^{\omega'}_{km}}{\mu^{\omega''}_{km}}=\infty
	\end{equation*}
	for all $\omega'\in\tilde{\tilde{\Omega_k}}$ and all $\omega''\in\tilde{\tilde{\Omega_k}}\setminus\lbrace\omega'\rbrace$. However, this is shown to be impossible in the proof of Proposition~\ref{prop_bayesianlearningbigworldinfiniteN}. The result thus follows.

\end{proof}

\subsection{Proof of Corollary~\ref{coro_bigworlddisagreementinfiniteN}}
\begin{proof}
	Consider an example where $\lim_{N\rightarrow\infty}p_{N}^{\omega}=0$ for all $\omega$ and $u_{N}(\omega',\omega)=0$ for all $\omega$ and $\omega'\neq\omega$. As shown in Proposition~\ref{prop_bigworldignorance2infiniteN}, all sequences of updating mechanisms must ignore almost all actions when $k$ goes to infinity. Thus, $\lim_{k\rightarrow \infty}L_{k}^{*}=\lim_{k\rightarrow\infty}\sum_{\omega}u_{N(k)}(\omega,\omega)p_{N(k)}^{\omega}$ and all updating mechanisms are $\epsilon$-optimal for all $\epsilon\geq 0$. Thus, if individual $A$ adopts an updating mechanism with $d_k(m)=1$ for all $m$ and $k$, while individual $B$ adopts an updating mechanism with $d_k(m)=2$ for all $m$ and all $k$ such that $N(k)\geq 2$, then they must disagree with each other under all $\omega$ for all big enough $k$ such that $N(k)\geq 2$.
\end{proof}	

\subsection{Proof of Proposition~\ref{prop_smallworldmistakes}}
\begin{proof}
	The proof follows closely the proof of Proposition~\ref{prop_smallworld}. For individual $B$, fixing the state $\omega$, in the stationary probability distribution, we have at the two extreme memory states in branch $\omega'$,
	\begin{equation*}
		\begin{split}
			\mu^{\omega}_{\omega'\lambda}\left[\frac{1-\gamma}{\delta}\sum_{\omega''\neq\omega'}F^{\omega}(G^{\omega''})+\gamma\right]&=\mu^{\omega}_{\omega'(\lambda-1)}\left[(1-\gamma)F^{\omega}(G^{\omega'})+\frac{\gamma}{2}\right]\\
			\mu^{\omega}_{\omega'(\lambda-1)}&=\mu^{\omega}_{\omega'\lambda}\left[\frac{(1-\gamma)F^{\omega}(G^{\omega'})+\frac{\gamma}{2}}{\frac{1-\gamma}{\delta}\sum_{\omega''\neq\omega'}F^{\omega}(G^{\omega''})+\gamma}\right]^{-1}
		\end{split}
	\end{equation*}
	for all $\omega'$. Similarly, at memory state $\omega'(\lambda-1)$,
	\begin{equation*}
		\resizebox{1\hsize}{!}{$
			\begin{split}
				\mu^{\omega}_{\omega'\lambda}\left[\frac{1-\gamma}{\delta}\sum_{\omega''\neq\omega'}F^{\omega}(S^{\omega''})+\gamma\right]+\mu^{\omega}_{\omega'(\lambda-2)}\left[(1-\gamma)F^{\omega}(S^{\omega'})+\frac{\gamma}{2}\right]&=\mu^{\omega}_{\omega'(\lambda-1)}\left[\frac{1-\gamma}{\delta}\sum_{\omega''\neq\omega'}F^{\omega}(S^{\omega''})+(1-\gamma)F^{\omega}(S^{\omega'})+\gamma\right]\\
				\mu^{\omega}_{\omega'(\lambda-2)}\left[(1-\gamma)F^{\omega}(S^{\omega'})+\frac{\gamma}{2}\right]&=\mu^{\omega}_{\omega'(\lambda-1)}\left[\frac{1-\gamma}{\delta}\sum_{\omega''\neq\omega'}F^{\omega}(S^{\omega''})+\frac{\gamma}{2}\right]\\
				\mu^{\omega}_{\omega'(\lambda-2)}&=\mu^{\omega}_{\omega'(\lambda-1)}\left[\frac{(1-\gamma)F^{\omega}(S^{\omega'})+\frac{\gamma}{2}}{\frac{1-\gamma}{\delta}\sum_{\omega''\neq\omega'}F^{\omega}(S^{\omega''})+\frac{\gamma}{2}}\right]^{-1}
			\end{split}
			$}
	\end{equation*}
	Repeating the same procedures implies that for all $k=1,\cdots,\lambda-1$
	\begin{equation}
		\mu^{\omega}_{\omega'k}=\mu^{\omega}_{\omega'\lambda}\left[\frac{(1-\gamma)F^{\omega}(S^{\omega'})+\frac{\gamma}{2}}{\frac{1-\gamma}{\delta}\sum_{\omega''\neq\omega'}F^{\omega}(S^{\omega''})+\gamma}\right]^{-1}\left[\frac{(1-\gamma)F^{\omega}(S^{\omega'})+\frac{\gamma}{2}}{\frac{1-\gamma}{\delta}\sum_{\omega''\neq\omega'}F^{\omega}(S^{\omega''})+\frac{\gamma}{2}}\right]^{-(\lambda-k-1)}	
	\end{equation}
	and 
	\begin{multline}
		\resizebox{1\hsize}{!}{$
			\mu^{\omega}_{0}=\mu^{\omega}_{\omega'\lambda}\left[\frac{(1-\gamma)F^{\omega}(S^{\omega'})+\frac{\gamma}{2}}{\frac{1-\gamma}{\delta}\sum_{\omega''\neq\omega'}F^{\omega}(S^{\omega''})+\gamma}\right]^{-1}\left[\frac{(1-\gamma)F^{\omega}(S^{\omega'})+\frac{\gamma}{2}}{\frac{1-\gamma}{\delta}\sum_{\omega''\neq\omega'}F^{\omega}(S^{\omega''})+\frac{\gamma}{2}}\right]^{-(\lambda-2)}	\left[\frac{(1-\gamma)F^{\omega}(S^{\omega'})+\frac{\gamma}{N}}{\frac{1-\gamma}{\delta}\sum_{\omega''\neq\omega'}F^{\omega}(S^{\omega''})+\frac{\gamma}{2}}\right]
			$}
	\end{multline}
	Note that for all $\gamma\in(0,1)$
	\begin{equation*}
		\frac{(1-\gamma)F^{\omega}(S^{\omega})+\frac{\gamma}{2}}{\frac{1-\gamma}{\delta}\sum_{\omega''\neq\omega}F^{\omega}(S^{\omega''})+\frac{\gamma}{2}}>1.
	\end{equation*}
	\begin{equation*}
		\frac{(1-\gamma)F^{\omega}(S^{\omega})+\frac{\gamma}{2}}{\frac{1-\gamma}{\delta}\sum_{\omega''\neq\omega}F^{\omega}(S^{\omega''})+\frac{\gamma}{2}}>\frac{(1-\gamma)F^{\omega}(S^{\omega'})+\frac{\gamma}{2}}{\frac{1-\gamma}{\delta}\sum_{\omega''\neq\omega}F^{\omega}(S^{\omega''})+\frac{\gamma}{2}}.
	\end{equation*}
	Then the result follows from the same steps in the proof of Proposition~\ref{prop_smallworld}.
\end{proof}

\bibliographystyle{econ}
\bibliography{reference_big}
\end{document}
